# Supplementary material for: Trustworthy Privacy-preserving Hierarchical Ensemble and Federated Learning in Healthcare 4.0 with Blockchain
Source: arXiv:2305.09209 source file (2023-05-16)
Supplement: Supplementary file 1 [file 06-appendix.tex]

\appendices

\section{}
Appendix one text goes here.

\section{}
Appendix two text goes here.
